# Supplementary material for: FashionDPO:Fine-tune Fashion Outfit Generation Model using Direct Preference Optimization
Source: arXiv:2504.12900 source file (2025-04-17)
Supplement: Supplementary file 1 [file Appendix.tex]

\clearpage
\setcounter{page}{1}

\section*{\centering Supplementary Material}

\setcounter{section}{0}

\textbf{Overview:In section \ref{sec:implementation_details}, we provide a more detailed explanation of each step in the experiment. In section \ref{sec:user_study}, we further introduce the human evaluation details. 
And in section \ref{sec:expert}, we analyze the different fashion experts based on the score distribution.
Finally, we illustrate more generation results in Section \ref{sec:results}.
}

\section{Implementation Details} \label{sec:implementation_details}
To ensure the reproducibility of the model, we describe the experimental details as comprehensively as possible here. We will outline the three components of the FashionDPO framework as follows:
1) fashion image generation without feedback, 2) feedback generation from multiple experts, and 3) model fine-tuning with direct preference optimization.

\textbf{Fashion Image Generation without Feedback.}
Our training subset consists of 1,000 outfits randomly selected from the iFashion or Polyvore-U dataset. During the sampling phase, we generate 7 recommended items for each outfit as a candidate set. 
The model initializes its parameters using the pre-trained DiFashion.
The sampling process is divided into 50 time steps within the set {1, 2, ..., 1000}. At each time step, we save the latent variables and the noise predicted by diffusion model as data for fine-tuning.

\textbf{Feedback Generation from Multiple Experts.}
We locally deploy MiniCPM to evaluate quality. For Compatibility, we train a VBPR model using paired outfit data from the POG and Polyvore-U dataset. Personalization is evaluated using the CLIP Score. Based on the score results, we categorize the preference pairs using a threshold.

1) \textbf{Quality:} We have deployed MiniCPM locally to evaluate the generated results, and the prompt used is: "Consider whether the fashion elements in the image are complete and whether they conform to fashion design principles. The goal is to classify the quality into one of the following categories: 1-Very Poor Quality, 2-Poor Quality, 3-Low Quality, 4-Below Average Quality, 5-Moderate Quality, 6-Above Average Quality, 7-Good Quality, 8-Very Good Quality, 9-High Quality, 10-Exceptional Quality. Please provide the best possible category based on the available information."

2) \textbf{Compatibility:} We trained the VBPR model using the iFashion dataset. Specifically, for each outfit in the dataset, we randomly selected one fashion item as the candidate image and the remaining three fashion items as the matching images. The training objective was to predict the compatibility between the candidate image and the matching images. We used ResNet to extract features for each fashion item, and averaged the three feature vectors from the matching images. We trained the model for 200 epochs on the entire dataset. When evaluating the VBPR model, we selected the generated images as the candidate images.

3) \textbf{Personalization:} We use the pre-trained CLIP (ViT-B/32) to encode the generated fashion items and user interaction history image items, and calculate the CLIP Score between them.

\textbf{Model Fine-tuning with Direct Preference Optimization.}
After the previous sampling and generated feedback, the FashionDPO framework constructs preference relationships within 7 items of 1000 sets of outfits.
In each outfit, if any two items from the 7 candidate generated items form a preference-non-preference relationship, we perform LoRA fine-tuning on the 50 saved timesteps. At each time step, we compute the loss $\mathcal{L}_{\mathrm{DPO}}$ and update the gradients.
Repeat this process until the preferences in each outfit have been learned by the model, thus completing one epoch. 
In the next epoch, a new subset of 1000 outfits is selected from the iFashion or Polyvore-U dataset as the training subset, and the "sampling fashion items - get multi-expert's feedback - fine-tuning" process is repeated. In our experiment, we fine-tuned DiFashion for five epochs to obtain the final fine-tuned model.

\section{Human Evaluation Details} \label{sec:user_study}
We collaborate with fashion design researchers to develop a specialized evaluation protocol that assesses the compatibility between generated images and incomplete outfits. The involvement of fashion experts, particularly those specializing in fashion design, is justified for two primary reasons:
(1) Evaluating the aesthetic coherence of clothing pairs can be subjective and prone to bias when conducted by individuals without formal fashion education. In contrast, fashion experts, with their rigorous training, can provide more objective and professional assessments by adhering closely to the evaluation criteria.
(2) Researchers in fashion design possess the expertise to create evaluation protocols suited for research-focused assessments rather than industry-level applications. This ensures that the protocol strikes a balanced approach—neither as stringent as evaluating designer artworks nor as simplistic as assessing commercial implementations.
Driven by these considerations, the fashion experts devise an evaluation protocol that emphasizes two key aspects: the rationality and diversity.

%To validate the effectiveness of our approach, we collaborate and invite five professional fashion designers aged 18-30 to conduct expert-level human evaluations. We use a five-level scoring protocol to score 30 sets of results generated by 2 different models regarding to four aspects of D1-D4 (style, color, fabric, variety).

% 注意对experts的background介绍，以及采用了什么机制保证他们的评价结果是objective and consistent

The rationality of clothes matching effects typically focuses on three fashion elements, \ie \textit{style}, \textit{color}, and \textit{fabric}. 
First, \textit{style} means the generated fashion items should adhere to the common pairing rules. It is typically reflected in clothing, accessories, and overall outfit design, such as casual, elegant, or street styles.
Second, \textit{color} refers to the appropriate usage and combination of hues, including contrasting, monochromatic, and achromatic pairings. 
Finally, \textit{fabric} emphasizes that all the items in a matching set should be aligned to the same season in terms of the used fabric.

The diversity metric in clothing matching emphasizes that a well-designed mix-and-match model should generate a variety of matching pairs rather than producing repetitive combinations with limited variation. However, it is important to note that the diversity metric cannot function in isolation; it must align with other essential factors such as style, color, and fabric to ensure consistency and aesthetic appeal.

\begin{table}
  \centering 
  \caption{Expert evaluation indicator weight scoring.}
  \scalebox{0.75}{
  \begin{tabular}{c|ccccccc}
  \toprule Scale & Expert 1 & Expert 2 & Expert 3 & Expert 4 & Expert 5 & Total & Weight \\
  \midrule D1-Style & 4 & 2 & 4 & 3 & 4 & 17 & $24 \% $ \\
  D2-Color & 4 & 3 & 4 & 3 & 4 & 18 & $25 \% $ \\
  D3-Fabric & 3 & 2 & 4 & 3 & 3 & 15 & $21 \% $ \\
  D4-Variety & 4 & 4 & 4 & 4 & 5 & 21 & $30 \% $ \\
  \bottomrule
  \end{tabular}
}
  \label{tab:weight}
\end{table}

\begin{figure*}
  \centering
  \includegraphics[width=1.0\textwidth]{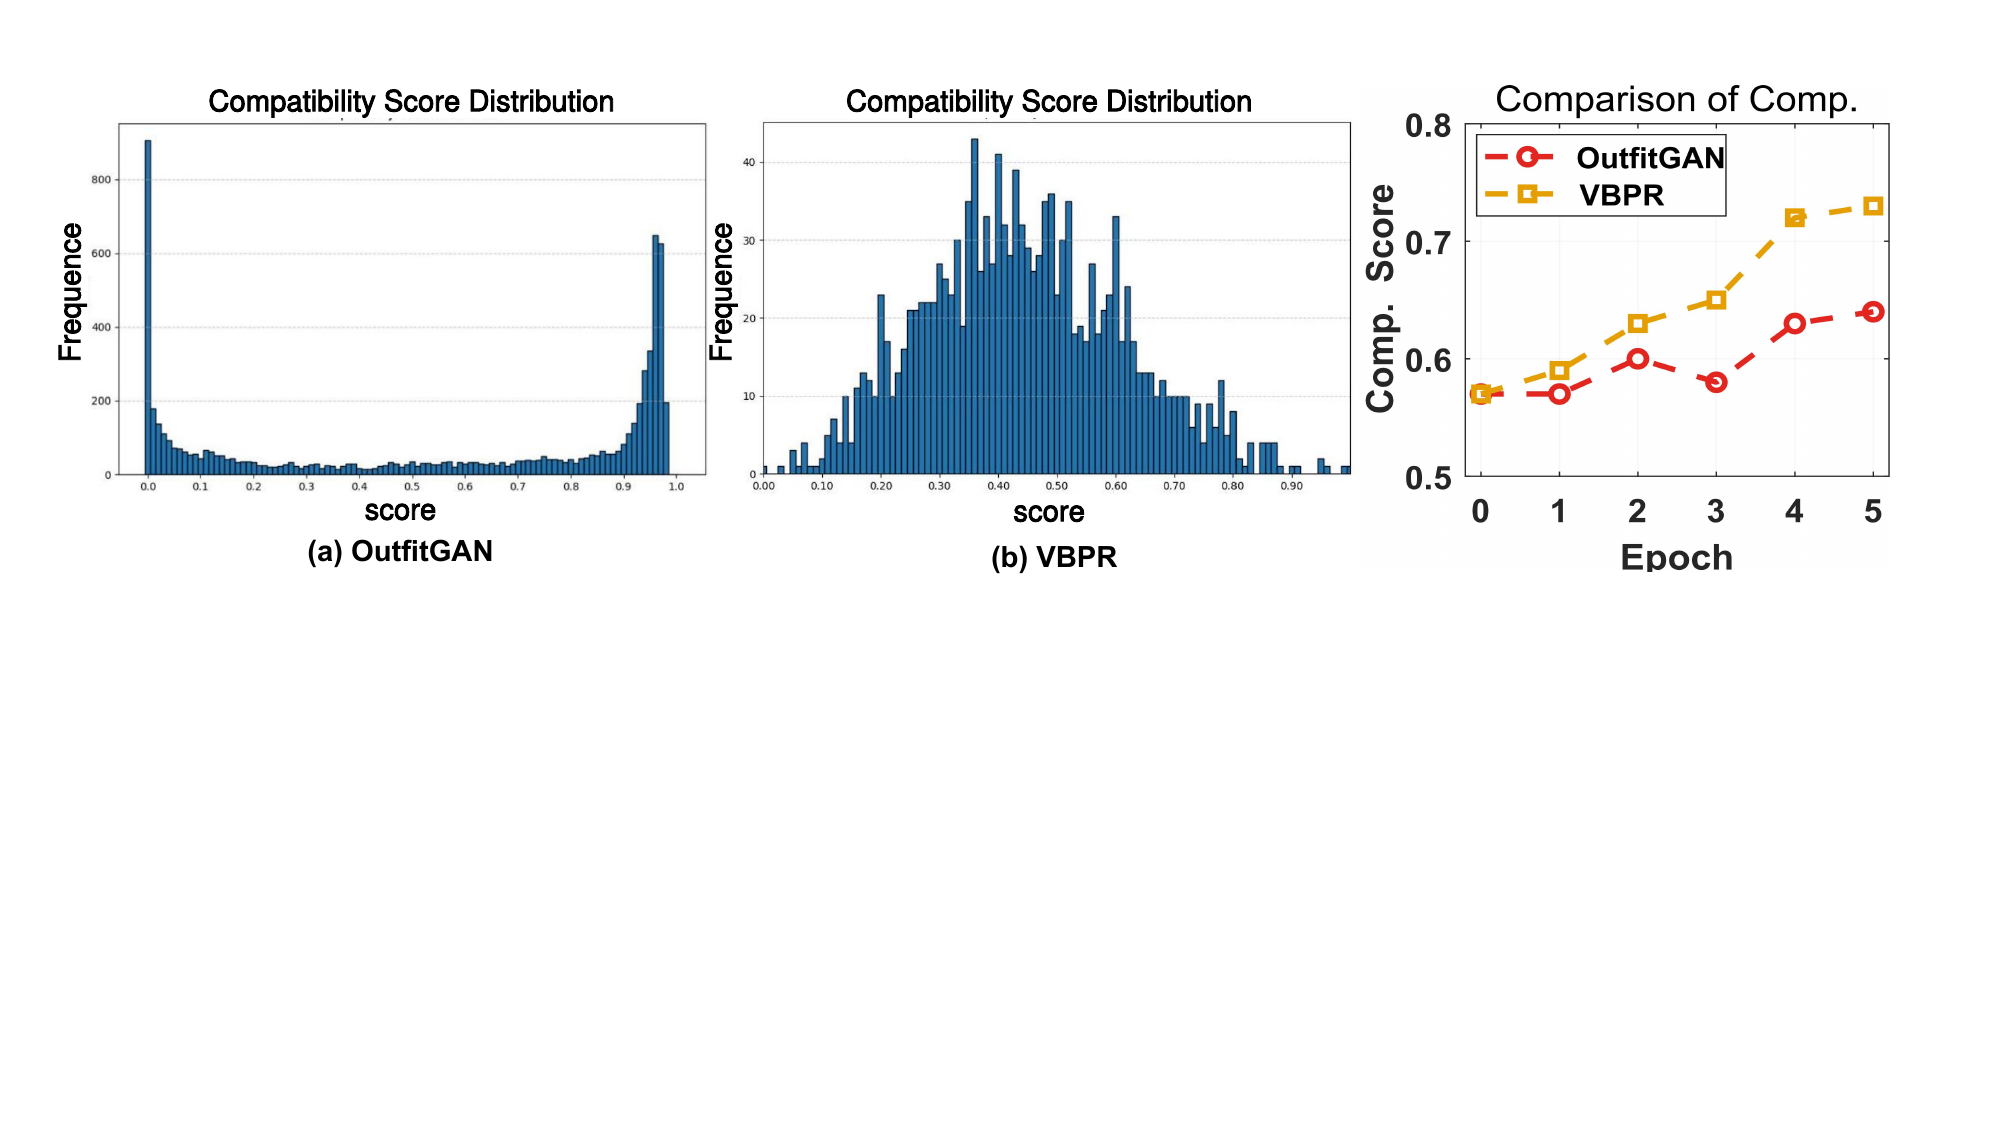}
  \caption{The score distributions when OutfitGAN and VBPR serve as compatibility experts.}
  \label{fig:suppl_expert}
\end{figure*}

To ensure that the evaluations from fashion experts are objective and consistent, we employed the fuzzy comprehensive evaluation method.
In this method, the weights reflect the importance of each criterion in the evaluation system, making it an extremely crucial factor in the assessment process. Therefore, whether the weights are scientifically and reasonably determined directly impacts the accuracy of the evaluation. Hence, we adopt the expert estimation method, combining the automatically generated matching characteristics to determine the weight distribution for four evaluation criteria: style, color, fabric, and diversity. As shown in the table \ref{tab:weight}, we invited five fashion experts who are knowledgeable about automatic generation technology to score four indicators on a five-level scale.

% \begin{table}
%   \centering 
%   \setlength{\tabcolsep}{2.pt}
%   \caption{Results of expert-level human evaluation.}
%   \vspace{-0.3cm}
%   \begin{tabular}{l|cccc}
%   \toprule Model & D1-Style & D2-Color & D3-Fabric & D4-Variety \\
%   \midrule DiFashion & 2.73±0.63 & 2.74±0.64 & 2.97±0.67 & 2.91±0.47\\
%   \textbf{FashionDPO(Ours)} & 4.08±0.52 & 3.87±0.37 & 3.63±0.50 & 3.22±0.43\\
%   \bottomrule
%   \end{tabular}
%   \label{tab:appendix_human_evaluation}
%   \vspace{-0.5cm}
% \end{table}

After determining the evaluation criteria and their weights, we organized fashion experts to assess 30*5 outfit combinations generated by two different models. Using a five-point rating scale, they evaluated the combinations from four aspects: style, color, material, and diversity. The rating categories included five levels of preference: very satisfied, satisfied, neutral, dissatisfied, and very dissatisfied, corresponding to scores from 5 to 1, respectively. The evaluation was conducted both online and offline. Finally, we collect valid scoring results from five designers for analysis. 
%The results of the questionnaire statistics are shown in Table ~\ref{tab:appendix_human_evaluation}.

Furthermore, we utilize variance analysis to investigate the differences between our FashionDPO and DiFashion. In variance analysis, the F-value is a statistic used to measure the ratio of between-group variance to within-group variance. A larger F-value indicates that the between-group variance is greater relative to the within-group variance, suggesting more significant differences between groups. The F-values for the two models across D1 to D4 are [81.175, 68.779, 18.386, 7.114], indicating that the fine-tuned model, FashionDPO, shows differences in various evaluation aspects compared to DiFashion. This demonstrates that the model has learned external fashion knowledge embedded in the expert feedback during the fine-tuning process.

\section{Expert Implementation} \label{sec:expert}

In the model study, we discuss the alternative implementations of experts. When we replace VBPR with OutfitGAN as the compatibility expert, the model's performance declines. To further investigate the reason, we conduct the following analysis on OutfitGAN:

The discriminator of OutfitGAN computes the compatibility score between the generated fashion item and the incomplete outfit, and the score is normalized through a sigmoid function. After VBPR calculates the predicted compatibility score, we apply min-max normalization to the score within the (0,1) range to observe its distribution.

As shown in Figure \ref{fig:suppl_expert}, the distribution of OutfitGAN is mainly concentrated around 0.0 and 1.0, indicating that OutfitGAN tends to make extreme judgments, either considering an outfit highly compatible or completely incompatible, with fewer scores in the middle range. The VBPR distribution, on the other hand, exhibits a near-normal shape, tending to assign moderate scores, resulting in a relatively balanced evaluation.
This indicates that OutfitGAN suffers from overfitting, with poor robustness and generalization ability.
Based on the training line chart, the compatibility score of OutfitGAN increases slowly with the number of epochs, indicating that it may require more training epochs or better hyperparameter tuning to achieve optimal performance. The VBPR, on the other hand, shows a smoother training process, suggesting that it is more stable during training and converges more easily to a good solution. This experiment demonstrates that the discriminative ability of the expert influences the effectiveness of fine-tuning. The more fashion knowledge the fashion expert possesses, the more accurate their judgments will be, leading to better improvements in the corresponding aspects of the fine-tuned model.

\section{Additional Results} \label{sec:results}

To demonstrate the capability of our fine-tuning framework in improving the quality, compatibility, and personalization of the generated results, we present additional generated samples. 
In Figure \ref{fig:suppl_result}, we show a comparison between the results generated by our model and those produced by the current SOTA method, DiFashion.
For example, in the first row, FashionDPO generates a wider variety of styles and patterns, producing skirts in different designs and materials, such as denim skirts, plaid skirts, and multi-layered pleated skirts. In contrast, DiFashion’s results focus primarily on a single type of skirt with similar textures.
Similarly, in the second row, FashionDPO also demonstrates a greater variety of styles, including diverse shapes and colors of earrings (such as red geometric designs, star-shaped pendants, and metal hoops).
In terms of compatibility, FashionDPO selects light-colored earrings that are more suitable for casual occasions, further enhancing the overall coherence of the outfit. In contrast, DiFashion generates earrings with colors that are too dark, making them unsuitable for pairing with the casual-style skirts.

% Nevertheless, the two methods show relatively similar performance in casual and sportswear outfits, with more room for improvement in the material variation of women's casual and sportswear styles. I

\begin{figure*}
  \centering
  \includegraphics[width=1.0\textwidth]{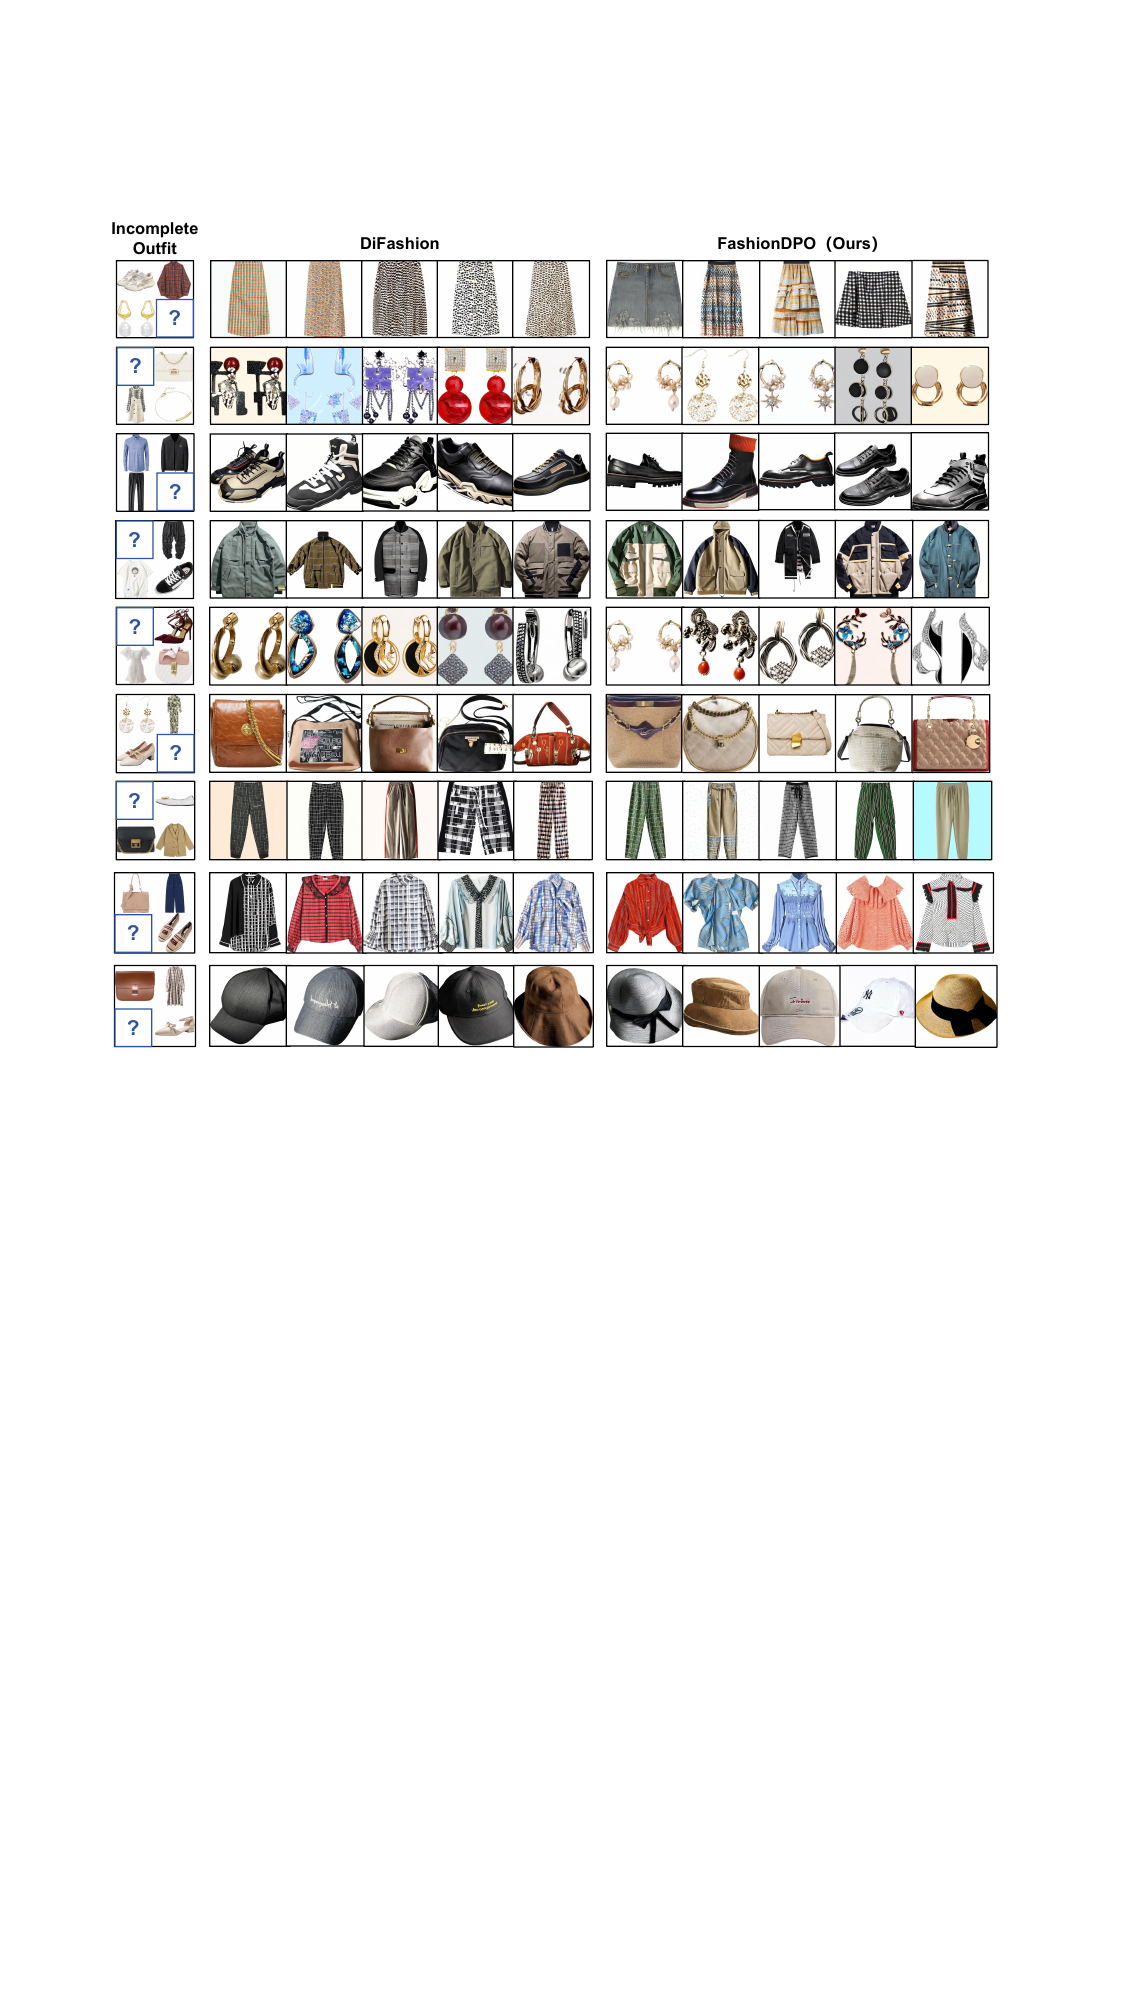}
  \caption{More results of the generated fashion items. It can be observed that our fashionDPO can generate images with diverse styles and improved matching combinations.
  }
  \label{fig:suppl_result}
\end{figure*}
